# Supplementary material for: Predicting Depth, Surface Normals and Semantic Labels with a Common Multi-Scale Convolutional Architecture
Source: arXiv:1411.4734 source file (2015-12-17)
Supplement: Supplementary file 1 [file supp.tex]

\begin{table*}[h]
\centering

\begin{tabular}{cc}

{
\tiny
\setlength{\tabcolsep}{4pt}
\begin{tabular}{|l|cccc|}
\hline
\multicolumn{5}{|c|}{\scriptsize {\bf 4-Class} (pixel acc.)} \\
\hline
\hline
& floor & struct & furntr & prop \\
\hline
Couprie \etal &   87.3 & 86.1 & 45.3 & 35.5 \\
Khan  \etal   &  87.1 &  88.2 & 54.7 & 32.6 \\
Stuckler \etal & 90.7 &  81.4  & 68.1  & 19.8 \\  
Mueller \etal &  {\bf 94.9} &  78.9  & 71.1  & 42.7 \\
Ours & 93.9 & {\bf 87.9} & {\bf 79.7} & {\bf 55.1} \\
\hline 
\end{tabular}
}

&

{
\tiny
\setlength{\tabcolsep}{4pt}
\begin{tabular}{|l|ccccccccccccc|}
\hline
\multicolumn{14}{|c|}{\scriptsize {\bf 13-Class} (pixel acc.)} \\
\hline
\hline
& bed & books & ceiling & chair & floor & furniture & objects & picture & sofa & table & tv & wall & window  \\
\hline
Couprie \etal & 30.3 & 31.7 & 33.2 & 44.4 & 68.0 & 28.5 & 10.9 & 38.5 & 25.8 & 18.0 & 18.8 & {\bf 89.4} & 37.8 \\
Wang \etal    & 47.6 & 45.0 & 68.1 & 23.5 & 84.1 & 16.7 & 12.4 & 26.4 & 39.1 & 35.4 & 32.4 & 65.9 & 52.2 \\
Hermans \etal & {\bf 68.4} & {\bf 45.4} & {\bf 83.4} & 41.9 & 91.5 & 37.1 & 8.6  & 35.8 & 28.5 & 27.7 & {\bf 38.4} & 71.8 & 46.1 \\
Khan \etal    & 38.1 & 13.7 & 62.6 & -    & 87.3 & -    & -    & -    & 29.8 & 10.2 & 6.0  & 86.1 & 15.9 \\
Ours          & 57.7 & 39.9 & 77.6 & {\bf 71.1} & {\bf 95.9} & {\bf 64.1} & {\bf 54.9} & {\bf 49.4} & {\bf 45.8} & {\bf 45.0} & 25.2 & 87.9 & {\bf 57.6}  \\
\hline
\end{tabular}
}

\end{tabular}

{
\tiny
\setlength{\tabcolsep}{4pt}
\begin{tabular}{|l|cccccccccccccccccccc|}
\hline
\multicolumn{21}{|c|}{\scriptsize {\bf 40-Class} (Jaccard index)} \\
\hline
\hline

 & bag          
 & bathtub      
 & bed          
 & blinds       
 & book         
 & bookshelf    
 & box          
 & cabinet      
 & ceiling      
 & chair        
 & clothes      
 & counter      
 & curtain      
 & desk         
 & door         
 & dresser      
 & floor        
 & floor-mat    
 & fridge       
 & lamp

\\

\hline

Gupta{\it \&al}'13

 & 0.65             
 & 33               
 & 55         
 & 44         
 & 4.4              
 & 20               
 & 4.8        
 & 48         
 & 59               
 & 40               
 & 6.9              
 & 47               
 & 34         
 & 10               
 & 8.3              
 & 22         
 & 81               
 & 22               
 & 15         
 & 6.8              

\\

Gupta{\it \&al}'14

 & 0.2              
 & {\bf 38.2}             
 & {\bf 65.0}             
 & 42.0             
 & 18.1             
 & 6.4              
 & 2.1              
 & 44.9             
 & 60.5             
 & {\bf 47.9}             
 & 4.7              
 & 51.3             
 & 29.1             
 & 11.3             
 & 20.3             
 & {\bf 34.8}             
 & 81.3             
 & 28.0             
 & 14.5             
 & {\bf 34.8}

\\

Ours 

 &  1.5     
 &  29.1    
 &  51.9    
 &  43.9    
 &  16.6    
 &  31.5    
 &  4.5     
 &  45.0    
 &  {\bf 75.2}    
 &  46.0    
 &  12.9    
 &  53.4    
 &  35.4    
 &  11.3    
 &  17.6    
 &  26.3    
 &  83.3    
 &  27.4    
 &  15.7    
 &  33.6    

\\

Ours (VGG)

 &  {\bf 2.0}  
 &    37.3  
 &    58.6  
 &  {\bf 50.7}  
 &  {\bf 20.0}  
 &  {\bf 36.4}  
 &  {\bf 6.6}  
 &  {\bf 51.6}  
 &    66.0  
 &    47.5  
 &  {\bf 14.1}  
 &  {\bf 57.1}  
 &  {\bf 37.3}  
 &  {\bf 12.6}  
 &  {\bf 28.7}  
 &    24.3  
 &  {\bf 84.1}  
 &  {\bf 29.8}  
 &  {\bf 26.0}  
 &    31.2

\\

\hline
\hline

 & mirror          
 & night-stand     
 & paper           
 & person          
 & picture         
 & pillow          
 & shelves         
 & showerctn       
 & sink            
 & sofa            
 & table           
 & toilet          
 & towel           
 & tv              
 & wall            
 & whitebd         
 & window          
 & other-furntr    
 & other-prop      
 & other-struct    
                   
\\

\hline

Gupta{\it \&al}'13

 & 19           
 & 20           
 & 1.9          
 & 16           
 & 40           
 & 28           
 & 5.1          
 & 18           
 & 26           
 & 44     
 & 30     
 & 50     
 & 14           
 & 9.3          
 & 68     
 & 37     
 & 33     
 & 2            
 & 22           
 & 6.9    

 \\

Gupta{\it \&al}'14

 & 16.4         
 & {\bf 27.2}         
 & 14.3         
 & 0.2          
 & 40.3         
 & {\bf 34.4}         
 & 3.5          
 & 4.2          
 & 37.5         
 & 47.9         
 & 29.9         
 & {\bf 55.1}         
 & 16.3         
 & 31.0         
 & 68.0         
 & 14.2         
 & 32.6         
 & 6.1          
 & 23.1         
 & 7.1          

 \\

Ours

 &  {\bf 32.6}     
 &  24.2     
 &  20.3     
 &  27.5     
 &  45.0     
 &  31.0     
 &  8.9      
 &  {\bf 21.7}     
 &  39.4     
 &  40.4     
 &  32.0     
 &  44.8     
 &  14.8     
 &  32.3     
 &  68.2     
 &  6.6      
 &  33.0     
 &  6.8      
 &  {\bf 29.4}     
 &  11.7     

\\

Ours (VGG)

 &   23.3   
 &   24.7   
 & {\bf 21.2}   
 & {\bf 37.8}   
 & {\bf 48.5}   
 &   33.4   
 &  {\bf 9.1}   
 &   20.2   
 & {\bf 41.3}   
 & {\bf 49.1}   
 & {\bf 35.7}   
 &   44.0   
 & {\bf 20.0}   
 & {\bf 35.9}   
 & {\bf 71.1}   
 & {\bf 39.7}   
 & {\bf 37.4}   
 & {\bf 8.8}   
 &   28.7   
 & {\bf 13.1}

\\

\hline
\end{tabular}
}

\label{tab:perclass}
\vspace{-3mm}
\end{table*}
